# Supplementary material for: Small Area Estimation using EBLUPs under the Nested Error Regression Model
Source: arXiv:2210.09502 source file (2022-10-18)
Supplement: Supplementary file 1 [file Supplementary_for_SAE.pdf]

# Supplementary material for “Small Area Estimation using EBLUPs under the Nested Error Regression Model”

June 29, 2022

## The Prasad-Rao mean squared error estimator

Let $\mathbf{X}_{(s)} = [\mathbf{X}_{(s)1}^T, \ldots, \mathbf{X}_{(s)g}^T]^T$, where $\mathbf{X}_{(s)i} = [\mathbf{x}_{ij}, j \in s_i]^T$, and $\mathbf{y}_{(s)} = [\mathbf{y}_{(s)1}^T, \ldots, \mathbf{y}_{(s)g}^T]^T$, where $\mathbf{y}_{(s)i} = [y_{ij}, j \in s_i]^T$, $\mathbf{Z}_{(s)} = \text{block diag}[\mathbf{1}_{s_1}, \ldots \mathbf{1}_{s_g}]$ with $\mathbf{1}_{n_i}$ the $n_i$-vector of ones, and $\mathbf{V}_{(s)} = \text{Var}(\mathbf{y}_{(s)}) = \text{block diag}[\dot{\sigma}_e^2 \mathbf{I}_{n_1} + \dot{\sigma}_\alpha^2 \mathbf{1}_{n_1}\mathbf{1}_{n_1}^T, \ldots, \dot{\sigma}_e^2 \mathbf{I}_{n_g} + \dot{\sigma}_\alpha^2 \mathbf{1}_{n_g}\mathbf{1}_{n_g}^T]$, with $\mathbf{I}_{n_i}$ the $n_i \times n_i$ identity matrix. Prasad & Rao (1990) showed that $\text{E}(\hat{M}_i^{\text{clp}} - \dot{\eta}_i)^2$, the unconditional MSE of $\hat{M}_i^{\text{clp}}$ for predicting $\dot{\eta}_i$, can be approximated to second order by

$$\text{MSE}_{\text{PR},i} = g_{1i}(\boldsymbol{\theta}) + g_{2i}(\boldsymbol{\theta}) + g_{3i}(\boldsymbol{\theta}) + o_p(g^{-1}),$$

where

$$\begin{aligned}
g_{1i}(\boldsymbol{\theta}) &= (1-\gamma_i)\sigma_\alpha^2, \\
g_{2i}(\boldsymbol{\theta}) &= \left(\bar{\mathbf{x}}_i - \gamma_i \bar{\mathbf{x}}_{i(s)}\right)^T \left(\mathbf{X}_{(s)}^T \mathbf{V}_{(s)}^{-1} \mathbf{X}_{(s)}\right)^{-1} \left(\bar{\mathbf{x}}_i - \gamma_i \bar{\mathbf{x}}_{i(s)}\right) \\
g_{3i}(\boldsymbol{\theta}) &= (1-\gamma_i)^2 \gamma_i \sigma_e^{-4} \sigma_\alpha^{-2} M(\boldsymbol{\theta}),
\end{aligned}$$

with $M(\boldsymbol{\theta}) = \sigma_\alpha^4 \text{Var}(\hat{\sigma}_e^2) + \sigma_e^4 \text{Var}(\hat{\sigma}_\alpha^2) - 2\sigma_\alpha^2\sigma_e^2 \text{Cov}(\hat{\sigma}_\alpha^2, \hat{\sigma}_e^2)$. The asymptotic variances and covariance of $\hat{\sigma}_\alpha^2$ and $\hat{\sigma}_e^2$ needed in $M(\boldsymbol{\theta})$ (i.e. under fixed or bounded small area size asymptotics) are given by

$$\text{Var}(\hat{\sigma}_\alpha^2) = 2w_1^{-2}\{(n-g-p+h)^{-1}(g-h)(n-p)\sigma_e^4 + 2w_1\sigma_\alpha^2\sigma_e^2 + w_2\sigma_\alpha^4\},$$

$$\text{Var}(\hat{\sigma}_e^2) = 2(n-g-p+h)^{-1}\sigma_e^4,$$

$$\text{Cov}(\hat{\sigma}_\alpha^2, \hat{\sigma}_e^2) = -(g-h)w_1^{-1}\text{Var}(\hat{\sigma}_e^2),$$

where $w_1 = n_{(s)} - \text{tr}\left\{(\mathbf{X}_{(s)}^T\mathbf{X}_{(s)})^{-1}\sum_{i=1}^g s_i^2\bar{\mathbf{x}}_{i(s)}\bar{\mathbf{x}}_{i(s)}^T\right\}$, $w_2 = \text{tr}\left[\left\{\mathbf{I}_{(s)} - \mathbf{X}_{(s)}(\mathbf{X}_{(s)}^T\mathbf{X}_{(s)})^{-1}\mathbf{X}_{(s)}^T\right\}\mathbf{Z}_{(s)}\mathbf{Z}_{(s)}^T\right]^2$, $\mathbf{I}_{(s)}$ denotes the $n_{(s)} \times n_{(s)}$ identity matrix, and $h = 0$ if the regression function (2.2) has no intercept term and $h = 1$ otherwise.

Using the second-order approximation, a second-order correct unbiased estimator of $\text{MSE}_{\text{PR}}$ (Prasad & Rao 1990 ) is given by

$$\widehat{\text{MSE}}_{\text{PR},i} = g_{1i}(\hat{\boldsymbol{\theta}}) + g_{2i}(\hat{\boldsymbol{\theta}}) + 2g_{3i}(\hat{\boldsymbol{\theta}}).$$

Based on the above approximation, a $100(1-\epsilon)\%$ prediction interval for $\dot{\eta}_i$ which we denote Syn-PR is

$$[\hat{M}_i^{\text{clp}} - \Phi^{-1}(1-\varepsilon/2)\widehat{\text{MSE}}_{\text{PR},i}^{1/2}, \hat{M}_i^{\text{clp}} + \Phi^{-1}(1-\varepsilon/2)\widehat{\text{MSE}}_{\text{PR},i}^{1/2}].$$

Table 1: Simulated relative design-bias and design RMSES of the point estimators Sam and Clp, together with the design-averages of the LW and PR estimators of their RMSEs for the consumer expenditure on fresh milk products in each state in 2002. The states are in the same order as in Table 3. * identifies states in Group 3 and † identifies states in Group 2.

| | ARB-Sam | ARB-Clp | AVE-LW | AVE-PR | RMSE-Sam-T | RMSE-Clp-T |
|---|---|---|---|---|---|---|
| 16 | -0.0135 | -0.0331 | 0.4401 | 0.4811 | 0.2228 | 0.1854 |
| 50† | -0.046 | -0.1088 | 0.4475 | 0.4797 | 0.4221 | 0.5396 |
| 31 | 0.0429 | 0.0842 | 0.4778 | 0.4798 | 0.2363 | 0.3348 |
| 22† | 0.0799 | 0.1494 | 0.4828 | 0.4797 | 0.2767 | 0.5091 |
| 21 | 0.0246 | 0.0473 | 0.4876 | 0.4804 | 0.1992 | 0.2155 |
| 15 | -0.0124 | -0.0222 | 0.4921 | 0.4805 | 0.2278 | 0.1865 |
| 32† | -0.0849 | -0.1446 | 0.4963 | 0.4801 | 0.498 | 0.7386 |
| 37† | 0.084 | 0.1468 | 0.5004 | 0.4797 | 0.3045 | 0.504 |
| 1 | 0.0013 | 0.0043 | 0.4094 | 0.4696 | 0.1308 | 0.1066 |
| 45 | 0.0016 | -0.0032 | 0.4133 | 0.47 | 0.2804 | 0.2246 |
| 2* | -0.075 | -0.1461 | 0.3877 | 0.4633 | 0.5044 | 0.8388 |
| 9* | 0.1442 | 0.2612 | 0.3779 | 0.462 | 0.4952 | 0.8517 |
| 41 | -0.01 | -0.0193 | 0.3719 | 0.4565 | 0.2307 | 0.169 |
| 49 | -0.0032 | -0.003 | 0.3553 | 0.4527 | 0.1975 | 0.1697 |
| 18 | 0.0193 | 0.0389 | 0.3455 | 0.448 | 0.2747 | 0.2248 |
| 27* | -0.0578 | -0.1188 | 0.3387 | 0.444 | 0.441 | 0.6954 |
| 8† | -0.0379 | -0.0699 | 0.326 | 0.4372 | 0.3475 | 0.3978 |
| 13 | 0.0049 | 0.0088 | 0.3095 | 0.4263 | 0.1908 | 0.1394 |
| 24† | 0.0519 | 0.1028 | 0.3045 | 0.4255 | 0.2645 | 0.4164 |
| 29 | 0.0167 | 0.0316 | 0.2982 | 0.4201 | 0.1411 | 0.1468 |
| 53 | -0.0119 | -0.0235 | 0.2937 | 0.4181 | 0.1553 | 0.141 |
| 55 | 0.0677 | 0.0884 | 0.4661 | 0.4608 | 0.2832 | 0.3305 |
| 51 | -0.0029 | -0.004 | 0.4681 | 0.4612 | 0.2004 | 0.1634 |
| 25 | -0.0111 | -0.0127 | 0.4508 | 0.4566 | 0.1716 | 0.1383 |
| 4 | -0.0141 | -0.0182 | 0.4456 | 0.4548 | 0.2259 | 0.2005 |
| 26 | 0.0323 | 0.0441 | 0.4317 | 0.45 | 0.2135 | 0.2116 |
| 34 | 0.0144 | 0.019 | 0.4043 | 0.4393 | 0.1968 | 0.1715 |
| 17 | 0.031 | 0.0401 | 0.4047 | 0.439 | 0.1896 | 0.189 |
| 39 | 0.0076 | 0.0115 | 0.3389 | 0.4041 | 0.1599 | 0.1398 |
| 42 | 0.0436 | 0.056 | 0.3173 | 0.3893 | 0.2186 | 0.2348 |
| 36 | -0.0028 | -0.0034 | 0.3056 | 0.3806 | 0.205 | 0.1814 |
| 12 | -0.0274 | -0.038 | 0.3033 | 0.3788 | 0.2162 | 0.2278 |
| 48 | 0.0209 | 0.0281 | 0.2934 | 0.3706 | 0.1861 | 0.1833 |
| 6 | -0.0179 | -0.025 | 0.2571 | 0.3375 | 0.1855 | 0.191 |
